# Supplementary material for: X-Learner: Learning Cross Sources and Tasks for Universal Visual Representation
Source: arXiv:2203.08764 source file (2022-03-16)
Supplement: Supplementary file 1 [file datasets.tex]

\section{Dataset Details}

In this section, we list 10 data sources used in the pre-training and 13 downstream datasets. All data are publicly available for non-commercial use.

\subsection{Pre-Training Datasets}

\noindent\textbf{ImageNet}~\cite{russakovsky2015imagenet} is a general classification dataset with 1.28M training data. Each image is labeled with one of the 1,000 classes.

\noindent\textbf{Places365}~\cite{zhou2017places} is a scene recognition dataset sampled from the Places database. We use the challenge version composed of 8 million training images comprising 365 scene classes. 

\noindent\textbf{iNat2021}~\cite{van2021benchmarking} is a large-scale image dataset collected and annotated by community scientists and contains over 2.7M images from 10k different natural species.

\noindent\textbf{CompCars}~\cite{yang2015large} contains data from two scenarios, including images from web-nature and surveillance-nature. We only use the former part with 163 car makes with 1,716 car models. We include all 136,726 images capturing entire cars, and predict their car make labels.

\noindent\textbf{Tsinghua Dogs}~\cite{zou2020new} is a fine-grained classification dataset for dogs, over 65\% of whose images are collected from real life. Each dog breed in the dataset contains at least 200 images and a maximum of 7,449 images.

\noindent\textbf{COCO}~\cite{lin2014microsoft} has 118k training images labeled with 80 object detection categories. 

\noindent\textbf{Objects365}~\cite{shao2019objects365} is a large-scale object detection dataset with 609k training data and 365 classes.

\noindent\textbf{WIDER FACE} dataset~\cite{yang2016wider} contains 32,203 images and 393,703 face labels with a high degree of variety in scale, pose and occlusion. For simplicity, we use the same mAP metric as COCO to report the pre-training performance on its validation set.

\noindent\textbf{ADE20K}~\cite{zhou2019semantic} has 20k images with 150 non-background classes covering scene categories from the SUN and Places databases.
%The dataset contains a wide variety of different indoor and outdoor scenes along with object classes.

\noindent\textbf{COCO-Stuff}~\cite{caesar2018cocostuff} is a dataset for scene understanding tasks like semantic segmentation and image captioning. It is constructed by annotating the original COCO images with additional stuff classes. There are 164k images spanning 172 categories including 80 things, 91 stuffs, and 1 unlabeled class.

\subsection{Downstream Datasets}

\noindent\textbf{CIFAR-10}~\cite{krizhevsky2009learning} is composed of 50k low-resolution training data labeled with 10 classes.

\noindent\textbf{CIFAR-100}~\cite{krizhevsky2009learning} is similar to CIFAR-10, but has 100 classes.

\noindent\textbf{Food-101}~\cite{downfood} consists of 101 food categories with 750 training and 250 test images per category, making a total of 101k images. The labels for the test images have been manually cleaned.
%, while the training set contains some noise.

\noindent\textbf{Oxford-IIIT Pets}~\cite{downpets} Dataset has 37 categories with roughly 200 images for each class. The images have large variations in scale, pose and lighting.

\noindent\textbf{Oxford 102 Flower}~\cite{downflowers} is an image classification dataset consisting of 102 flower categories. The flowers are chosen to be commonly occurring in the United Kingdom. Each class consists of between 40 and 258 images. %The images have large scale, pose and light variations. In addition, there are categories that have large variations within the category and several very similar categories.

\noindent\textbf{SUN397}~\cite{downsun} contains 899 classes and 130,519 images. There are 397 well-sampled categories to evaluate algorithms for scene recognition.

\noindent\textbf{Stanford Cars}~\cite{downcar} dataset consists of 196 classes of cars with a total of 16,185 images, taken from the rear. The data is divided into almost a 50-50 train/test split with 8,144 training images and 8,041 testing images.
% The images are 360×240.

\noindent\textbf{Describable Textures Dataset (DTD)}~\cite{downdtd} contains 5,640 texture images in the wild. They are annotated with human-centric attributes inspired by the perceptual properties of textures.

\noindent\textbf{Caltech-101}~\cite{downcaltech} dataset is composed of images from 101 object categories and one additional background class.
% and a background category that contains the images not from the 101 object categories.
% For each object category, there are about 40 to 800 images, while 
Most classes have about 50 images.
%The resolution of the image is roughly about 300×200 pixels.

\noindent\textbf{FGVC-Aircraft}~\cite{downaricraft} contains 10,200 images of aircraft, with 100 images for each of the 102 different aircraft model variants, most of which are airplanes. 

\noindent\textbf{PASCAL Detection}~\cite{Everingham10VOC} refers to the PASCAL VOC object detection dataset with 20 object classes. We use the VOC07+12 set with 16.5k data for training, and evaluate on the PASCAL VOC 2007 test set.

\noindent\textbf{PASCAL Segmentation}~\cite{Everingham10VOC} denotes the PASCAL VOC 2012 segmentation dataset with 1.5k training images and 20 classes.

\noindent\textbf{NYU-Depth V2}~\cite{silberman2012indoor} is a depth estimation dataset. It contains 120K RGB and depth pairs acquired as video sequences using a Microsoft Kinect from 464 indoor scenes. We follow the BTS~\cite{bts} split, using 249 scenes (24,231 images) for training and 215 scenes (654 images) for testing.
