# Supplementary material for: X-Learner: Learning Cross Sources and Tasks for Universal Visual Representation
Source: arXiv:2203.08764 source file (2022-03-16)
Supplement: Supplementary file 2 [file cls.tex]

\section{Linear Probe in Classification}

\begin{figure*}[ht]
\centering
 \includegraphics[width=1.0\linewidth]{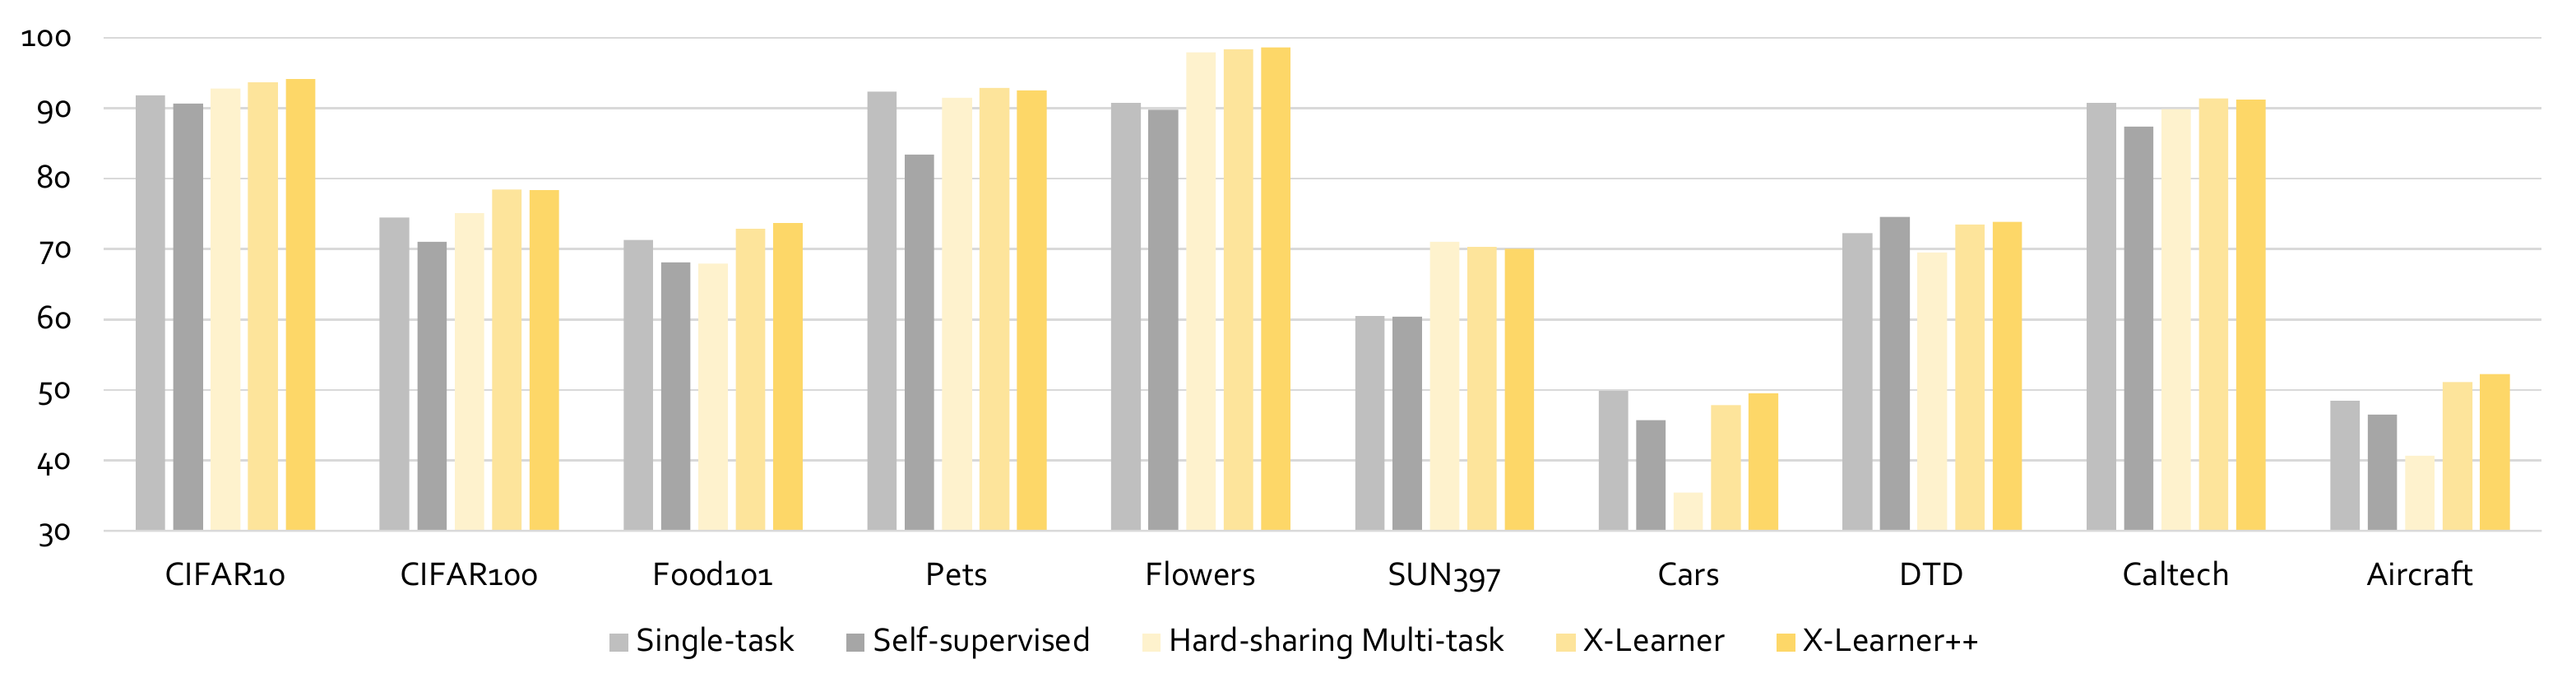}
 \caption{\textbf{Linear probe performance on transfer data of main experiments. }}
 \label{fig:detail_result_cls}
\end{figure*}

The  detail results of each dataset in linear evaluation are shown in~\cref{fig:detail_result_cls}.
