# Supplementary material for: X-Learner: Learning Cross Sources and Tasks for Universal Visual Representation
Source: arXiv:2203.08764 source file (2022-03-16)
Supplement: Supplementary file 3 [file half_r50.tex]

\section{HalfResNet-50 Used in \framework{}$_{\boldsymbol{r}}$}

%%%%%%%%%%%%%%%%%%%%%%%%%%%%%%%%%%%%%%%%%%%%%%%%%%%%%%%%%%%%%%%%%%
%  Half-ResNet 参数对比表
%%%%%%%%%%%%%%%%%%%%%%%%%%%%%%%%%%%%%%%%%%%%%%%%%%%%%%%%%%%%%%%%%%
\begin{table}
\centering
\resizebox{8cm}{!}{%
\begin{tabular}{c	|	c	|	c}
\toprule
Model & ResNet-50 & HalfResNet-50 \\
\hline
Channels & (256, 512, 1024, 2048)
 &  (180, 360, 724, 1448) \\
\hline 
Parameters & 23,508,032 & 11,761,825 \\
\bottomrule
\end{tabular}
}
\caption{\label{tab:half-r50} The number of parameters and channel configuration of ResNet-50 and HalfResNet-50. }
\end{table}
%%%%%%%%%%%%%%%%%%%%%%%%%%%%%%%%%%%%%%%%%%%%%%%%%%%%%%%%%%%%%%%%%%
% END
%%%%%%%%%%%%%%%%%%%%%%%%%%%%%%%%%%%%%%%%%%%%%%%%%%%%%%%%%%%%%%%%%%

% We show the results of \framework{}$_{r}$ in~\cref{fig:stage3-experiment-module}. 
For implementing X-Learner$_{r}$, we use a HalfResNet-50 as sub-backbone with only $ 1 / \sqrt{2} $ of the original ResNet-50 channels (see \cref{tab:half-r50} for details).
% The amount of parameter in expand X-Learner$_{r}$ is strictly no bigger than the amount of ResNet-50.
