# Supplementary material for: X-Learner: Learning Cross Sources and Tasks for Universal Visual Representation
Source: arXiv:2203.08764 source file (2022-03-16)
Supplement: Supplementary file 4 [file must.tex]

\section{Comparison with MuST}

%\resizebox{\linewidth}{!}
%{
% \begin{tabular}{lccccc}
% \toprule
% \multicolumn{1}{l|}{Method} &   AVG Cls & CIFAR-100~\cite{krizhevsky2009learning}               & PASCAL Det~\cite{Everingham10VOC}          & PASCAL Seg~\cite{Everingham10VOC}     & NYU-Depth V2~\cite{silberman2012indoor}      \\ \hline
% \multicolumn{1}{l|}{MuST~\cite{MuST2021}} & -- & 86.3& 85.1& 80.6 & 87.8 \\ \hline
% % \multicolumn{1}{l|}{COCO Supervised}          & R50  & 67.6                   & 82.2                          & 84.7                   & run*                  \\
% \multicolumn{1}{l|}{X-Learner$_\text{R152}$} & 78.2 & \textbf{89.7} \textcolor{blue}{(+3.4)}& \textbf{88.6} \textcolor{blue}{(+3.5)}& \textbf{82.6} \textcolor{blue}{(+2.0)} & \textbf{91.3}\textcolor{red}{*}   \textcolor{blue}{(+3.5)}\\
% \bottomrule
% \end{tabular}
% %}
\begin{table*}
\label{tab:r152}
\centering
\small
\caption{\textbf{Comparison with MuST.} We use the same pre-training datasets as MuST without MiDaS~\cite{midas}. Our setting can take advantage of most existing vision datasets. We replace the sub-backbone of X-Learner with ResNet-152. \textcolor{red}{*} represents that depth estimation (NYU-Depth V2) is an unseen task for X-Learner, but it is included in the training process of MuST.}
\resizebox{1.0\linewidth}{!}
{
\begin{tabular}{lc|c|cccc}
\toprule
\multicolumn{1}{l|}{Method}& Backbone & Pre-training Settings & CIFAR-100~\cite{krizhevsky2009learning}     & PASCAL Det~\cite{Everingham10VOC} & PASCAL Seg~\cite{Everingham10VOC}   & NYU-Depth V2~\cite{silberman2012indoor}      \\ \hline
\multicolumn{1}{l|}{MuST~\cite{ghiasi2021multi}}  & ResNet-152 & ImageNet + OBJ365 + COCO + MiDaS & 86.3& 85.1& 80.6 & 87.8\\ 
\multicolumn{1}{l|}{MuST~\cite{ghiasi2021multi}}  & ResNet-152 & JFT300M + OBJ365 + COCO + MiDaS & 88.3& 87.9& \textbf{82.9} & 89.5\\ 
% \multicolumn{1}{l|}{COCO Supervised}          & R50  & 67.6                   & 82.2                          & 84.7                   & run*                  \\
\multicolumn{1}{l|}{X-Learner$_{R152}$}  & ResNet-152 & ImageNet + OBJ365 + COCO   & \textbf{88.7} \textcolor{blue}{(+2.4)}& \textbf{88.5} \textcolor{blue}{(+3.4)}& \textbf{81.4} \textcolor{blue}{(+0.8)} & \textbf{91.2}\textcolor{red}{*}\textcolor{blue}{(+3.4)} \\
% \multicolumn{1}{l|}{X-Learner w/ seg FPN}   & TBD& TBD& TBD\\  
\bottomrule
% \multicolumn{1}{l|}{MuST}& R152 & -& 85.1& 80.6\\
% \multicolumn{1}{l|}{X-Learner}& R152 & TBD& TBD& TB\\ \hline
\end{tabular}
}
\end{table*}
% \vspace{-10pt}
% \vspace{-4mm}
% \end{table}

%while the depth data has been seemed in the training process.
% }

% Instead of training with ResNet-50 backbone, 
For fair comparison with MuST~\cite{ghiasi2021multi}, a self-training approach using ResNet-152 as the backbone, we also conduct the experiment with the same backbone and dataset (except for MiDaS~\cite{midas}). Table \ref{tab:r152} provides the performance comparison on four different downstream tasks. We observe that our framework outperforms MuST by significant margins over all evaluated downstream tasks. When compared with MuST pre-trained with JFT-300M, X-Learner$_\text{R152}$ shows the high data efficiency. 
% X-Learner outperforms the representation on each downstream task.
Moreover, it is worth mentioning that our X-Learner surpasses MuST on NYU-Depth V2 without any depth estimation pre-training. However, MuST takes MiDaS,  for pre-trainning which is large depth estimation dataset including 1.9M images. This zero-shot performance further demonstrates the strong generalization capability of X-Learner.
